# Supplementary material for: Efficiency through Uncertainty: Scalable Formal Synthesis for Stochastic Hybrid Systems
Source: arXiv:1901.01576 source file (2019-01-06)
Supplement: Supplementary file 1 [file appendix.tex]

% appendix
\appendix

The following result will be useful in the case studies.
\begin{proposition}
\label{BOundDiagonal}
Let $F$ be a diagonal matrix with negative diagonal entries. Assume $G$ is the identity matrix. Assume the safe set $\mathcal{S}$ is a hyper-rectangle centered at the origin. Then, for any $I=[0,h],h>0, q_i,q_j \in \mathcal{S}, x_i \in q_i, x_j \in q_j$ we have that $E_I^{i,j}=0$. 
\end{proposition}
\begin{proof}
Let $E_{\mathcal{B}}(t)$ the expectation of $\mathcal{B}=X|X(0)=x_i,X(h)=x_j$ at time $t$. Being $F,G$ diagonal, each component of $E_{\mathcal{B}}(t)$ is independent of the other, and they can be treated separately. Then, in order to prove the proposition is enough to show that for each $k\in \{0,...,m \},$ $\max\{|x_{i,k}-\partial \mathcal{S}|,|x_{j,k}-\partial \mathcal{S}|\}\geq |E_{\mathcal{B},k}(t)-\partial \mathcal{S}|$ for any $t \in [0,h]$, where $x_{j,k}$ is the $k-th$ component of vector $x_j$.
We have that
\begin{align}
\nonumber
&E_{\mathcal{B},k}(t)=\\
&\,\frac{(2 e^{F_kh}(x_{j,k} - x_{i,k}e^{F_k h})(sinh(F_k t))}{e^{2F_k h} - 1} + x_{i,k}e^{F_k t},
\label{BridgeExpectationDiagonal}
\end{align}
where $sin h(t)=\frac{(e^t-e^{-t})}{2}$ is the hyperbolic sin at time $t$ and $F_k$ is the $k-th$ element of the diagonal of $F$.
In order to prove the property is enough to show that for any $t\in [0,h],$ $|E_{\mathcal{B},k}(t)|\leq max\{|x_1|,|x_3| \}$.
Assume $x_{j,k}>x_{i,k}$ and $|x_{j,k}|>|x_{i,k}|$ and assume Proposition \ref{BOundDiagonal} does not hold. Then, there must exists $t\in (0,h)$ such that
$E_{\mathcal{B},k}(t)\geq x_{j,k}.$
The above equations admit two solution $t=h,$ which is not in $(0,h),$ and
$t=\frac{log(\frac{x_{j,k}-x_{i,k}e^{F_k h}}{x_{i,k}-x_{j,k}e^{F_k h}})}{f_k}.$
Being $f_k<0$, this is an admissible solution only for
$$ 0< \frac{x_{j,k}-x_{i,k}e^{F_k h}}{x_{i,k}-x_{j,k}e^{F_k h}})<1. $$
However, this cannot be satisfied for $|x_{j,k}|>|x_{i,k}|.$

Consider now the case $0\geq x_{j,k}> x_{i,k}$ and $|x_{i,k}|\geq |x_{j,k}|$. In this case, it must hold that $x_{i,k}<0$. Thus, if Proposition \ref{BOundDiagonal} does not hold there must exists a time $t\in (0,h)$ such that
$$\frac{(2 e^{F_kh}(x_{j,k} - x_{i,k}e^{F_k h})(sinh(F_k t))}{e^{2F_k h} - 1} + x_{i,k}e^{F_k t}\leq x_{i,k}.$$
This may admit solution only for $x_{j,k} - x_{i,k}e^{F_k h}<0.$ However this would imply
$$1\geq \frac{sinh(F_k t)}{sinh(F_k h)} \geq   \frac{x_{i,k} - x_{i,k}e^{F_k t}}{(x_{j,k} - x_{i,k}e^{F_k h})},$$
which is a contradiction as $\frac{x_{i,k} - x_{i,k}e^{F_k t}}{(x_{j,k} - x_{i,k}e^{F_k h})}>1 $ for $t<h.$

Similar reasoning can be applied for the case $x_1>x_3.$

%Call $s_k$ the component $k$ of the projection of one of the two vertices of $\partial\mathcal{S}$. Without any loss of generality assume $s_k>0$.
%Then, $s_k-x\geq 0$ for any $x\in \mathcal{S}.$
%Now
%\begin{align}
%&\frac{d s_k-E_{\mathcal{B},k}(t)}{h}=\\
%&\,-(\frac{(2(x_{i,k} - x_{j,k}*e^{-f_m h})(cosh(-f_k t))}{e^{-2f_k h} - %1} + f_k x_{i,k}e^{f_k t}),
%\end{align}
%THere are now two cases \\
%a) $(x_{i,k} - x_{j,k}e^{-f_m h})>0$

%In this case $\frac{d s_k-E_{\mathcal{B},k}(t)}{h}<0$ for any $t>0.$ Thus, the function is maximized in $x_i$.

%b)$(x_{i,k} - x_{j,k}e^{-f_m h})<0$

%In this case we can write $E_{\mathcal{B},k}(t)\geq\frac{(2(x_{i,k} - x_{j,k}e^{-f_m h})(sinh(f_k t))}{e^{-2f_k h} - 1} - x_{i,k}$.
%Thus, $$s_k-E_{\mathcal{B},k}(t)\geq s_k-\frac{(2(x_{i,k} - x_{j,k}e^{-f_m h})(sinh(f_k t))}{e^{-2f_k h} - 1} - x_{i,k}..$$
%It is easy to verify that the last term is maximized in $t=h$ (derivative always positive). And for $t=h,$ we have

%NO second term does not work. Just show it for the particular case study

\end{proof}
